# Supplementary material for: Adventures in Radio Astronomy Instrumentation and Signal Processing
Source: arXiv:1109.0416 source file (2011-09-02)
Supplement: Supplementary file 2 [file FlysEyeUGAppendix.tex]

\chapter{User Guide for the Fly's Eye Instrument}

Blah

\newpage
