# Supplementary material for: Adventures in Radio Astronomy Instrumentation and Signal Processing
Source: arXiv:1109.0416 source file (2011-09-02)
Supplement: Supplementary file 3 [file HPProCurveAppendix.tex]

\chapter{Benchmark Results from the HP ProCurve 2900}

Blah

\newpage
